# Supplementary material for: Optical spectra of silver clusters and nanoparticles of all sizes from the TDDFT+U method
Source: arXiv:2405.02910 source file (2024-05-05)
Supplement: Supplementary file 1 [file SI.pdf]

# Supplementary Material

## Optical spectra of silver clusters and nanoparticles of all sizes from the TDDFT+U method

**Mohit Chaudhary**[†,‡] **and Hans-Christian Weissker**[*,†,‡]

†Aix-Marseille University, CNRS, CINAM, Marseille 13288, France

‡European Theoretical Spectroscopy Facility (ETSF), www.etsf.eu

E-mail: hans-christian.weissker@univ-amu.fr

**1. Dielectric shifts and comparison with experiments on rare-gas-embedded clusters:** As mentioned above, the spectra of clusters in rare-gas matrices are not identical to those of clusters in vacuum due to the interaction with the matrices, even though this latter is generally considered to be weak. Most important for intermediate sizes and larger clusters is the dielectric shift due to the polarizable matrix. Fedrigo *et al.*[20] have studied small silver clusters in different rare gases and found increasing red-shifts, for example, for $Ag_{21}$ clusters in Ar, Kr, and Xe. For similar sizes, Yu *et al.*[5] have aligned measurements of intermediate sizes by using shifts of 0.17 eV for Ne and 0.29 eV for Ar.

For the smallest clusters, below about 11 atoms, the situation is more complicated. On the one hand, so-called site-isomers may occur, with slightly different spectra. In particular, the matrix effect has been described for small Na clusters in Ar by Gervais *et al.*[21] as originating on the one hand from the dielectric matrix, producing the red-shifts that we have discussed above, and second from confinement effects due to the Pauli repulsion between the Na electrons and the Ar atoms which, by contrast, lead to a blue shift. The overall effect is then determined by the respective weight of these two counteracting effects. For $Na_8$ in Ar, the two effects were found to cancel almost completely.[21] Consequently, it is reasonable to expect the overall shifts for very small clusters to be very small or zero. This is also corroborated by Lecoultre *et al.*[4] who measured Ag clusters in Ne and obtained very good agreement with theory using the B3LYP hybrid functional and no shifts.

In our general presentation, we follow the work by Yu *et al.*[5] and shift the plasmon energies of the intermediate-sized clusters by 0.17 eV (Ne) in Fig. 1 of the manuscript. The spectra of the smallest clusters (<20 atoms) are left unshifted as measured. In their work, TDDFT calculations employing an explicit Ne matrix have been compared with clusters in vacuum. While the overall results appear to be a validation of the matrix shifts, close inspection of the results shows that for the smallest cluster treated, $Ag_{20}$, the vacuum calculation lies slightly lower than the shifted environment calculation, whereas for the largest clusters, 92 atoms, it lies slightly higher. This could be an indication that indeed the shifts are not the same for all sizes and energies, and that in fact the spectra of the smallest clusters will not undergo any substantial shift.

The full treatment of the matrix-related shifts is clearly a very complex problem. Our work does not and cannot aspire to solve the problem of the shifts, but we need to be clear about the

limits of our comparison with experiment lest we draw false conclusions. In particular, we cannot take precise values of the shifts for granted nor their total absence in the case of the small clusters.

To obtain a clear idea of the limits of the comparison with experiment, we compare in Supplementary Fig. S1 our calculated spectra with the *shifted* spectra *and* with the *unshifted*, original spectra. In agreement with the discussion above, our results for the intermediate sizes lie mostly between the two limiting cases, whereas they agree well with the unshifted spectra for the smallest clusters. Thus, the comparison in Fig. S1 provides some sort of ``error bars'' for the comparison with our calculations. This has likewise inspired the representation of the energies in Fig. 3 of the manuscript.

**2. Possible reasons for the red-shift in free-beam experiments:** When comparing the calculations with the different free-beam experiments, it's important to note that only a part of the measurements are performed on size-selected clusters ([12] and the small clusters of Ref. [13]). For the non-size-selected measurements, a well-known bias deriving from the size distribution will be caused by the fact that the larger particles will contribute more to the spectra because of their higher volume/number of atoms. This will clearly induce a red-shift compared to the value valid for the center of the size distribution. Furthermore, Haberland[14] conjectures that the high internal temperatures (``boiling hot'') could play a role as well.[14,15] That idea is at least partially supported by recent calculations and measurements on embedded clusters which both suggest a red-shift of the plasmon energies with increasing temperature.[16,17] In addition, the clusters cannot simultaneously all be of high symmetry/approximately spherical and a substantial effect due to shape isomerism is expected, in particular at high temperatures.[18,22] The effect on the energies is difficult to estimate. In principle, it is the same effect as discussed below for the lowest-energy structure of $Ag_{58}$. While for a single structure, this will be reproduced by the calculations if the correct structure is used, the occurrence of multiple isomers will not. Moreover, for the smaller clusters, the charges cannot be neglected, leading to substantial red-shifts for negative charges. Finally, the results of Loginov *et al.*[19] have been measured in helium droplets which should also produce an - albeit small and not easy to estimate - red-shift, which is not included in Fig. 3 of the manuscript.

All these effects are expected to produce small red-shifts compared to the situation described in the calculations: defined nearly spherical clusters (without size distribution or isomerism) at zero temperature. Consequently, assuming that the TDDFT+U description is correct and precise, our calculations should produce plasmon energies within or slightly above the values measured in the various free-beam experiments. This is indeed what we find, as shown in Fig. 3 of the manuscript.

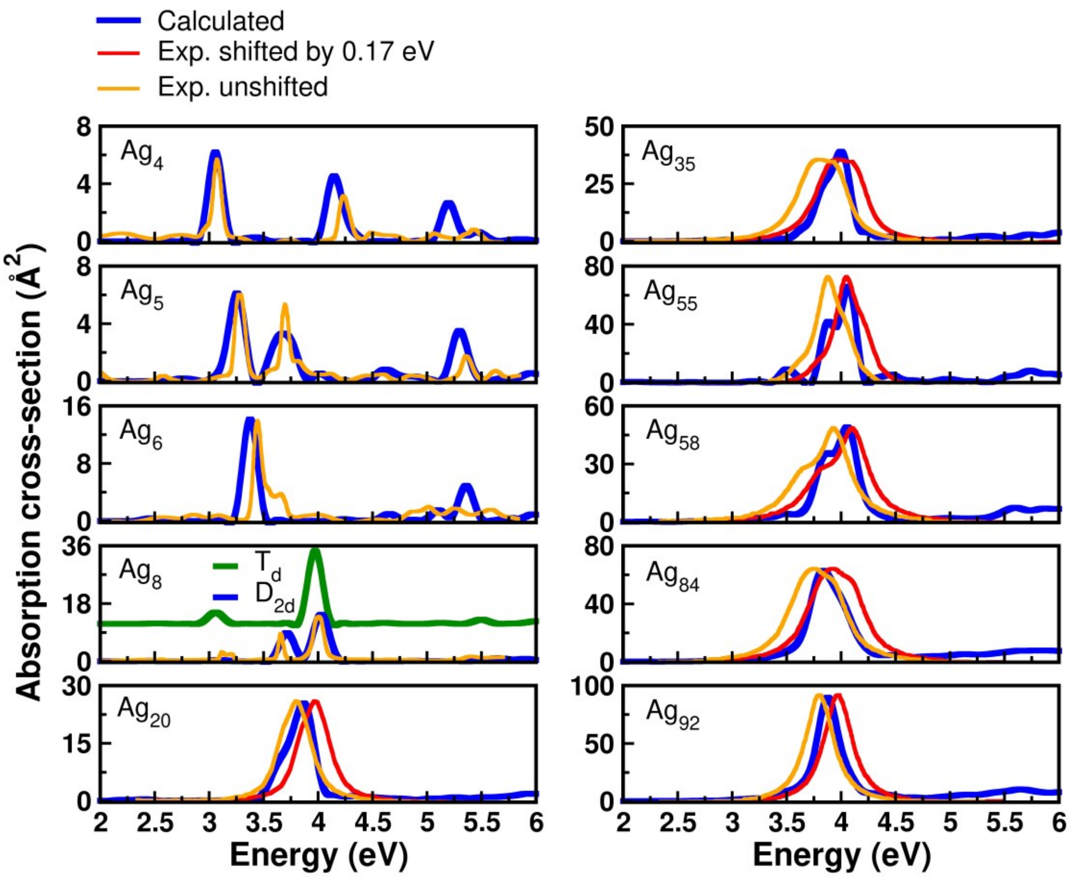


**S1:** Comparison of the calculated spectra with experiment, similar to Fig. 1 of the manuscript. To discuss the impact of the matrix-induced shifts as applied by several authors and discussed in the literature, we show for the clusters between sizes of 20 and 92 atoms the shifted spectra (red) along with the unshifted, raw spectra (orange). In most cases, our calculated spectra lie between the shifted and the unshifted spectra, which corresponds to the fact that in Fig. 3 of the main manuscript many of the plasmon energies lie within the band defined by the shifted and unshifted values. For the smallest clusters, our results agree well with the unshifted spectra, which has been the case also for the calculations using the B3LYP hybrid functional[4] and the range-separated hybrid functional.[2]

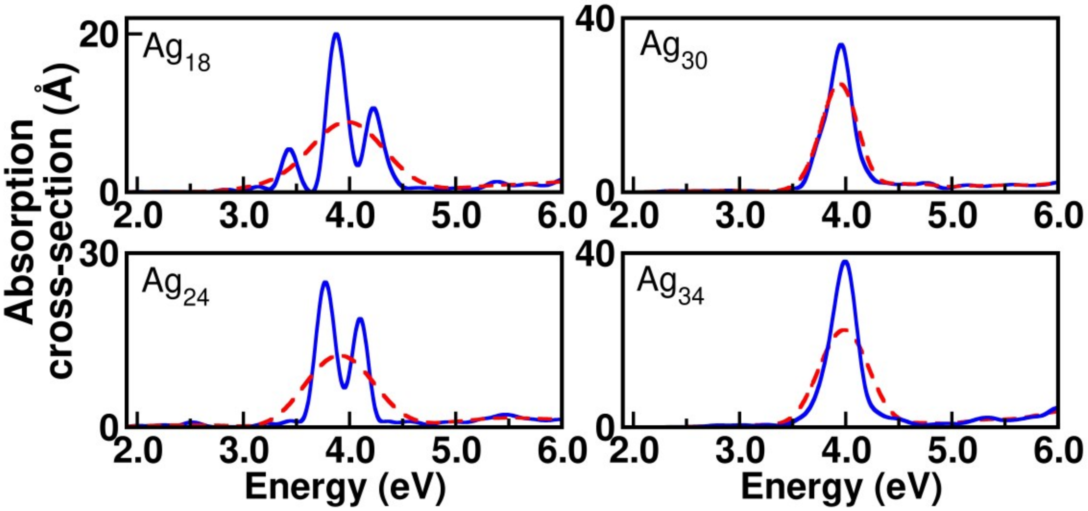


**S2:** Absorption spectra calculated using the lowest energy structure taken from the work of Chen *et al*.,[11] except for $Ag_{34}$, which was constructed by selectively removing an atom from the $Ag_{35}$ cluster (details provided in method section of the manuscript). The blue curve corresponds to the spectra obtained using TDDFT+U with an evolution time of ≈ 26 fs (40 $\hbar$/eV), and the red dashed curves are obtained with a shorter evolution time, which is equivalent to applying a larger broadening to spectra.

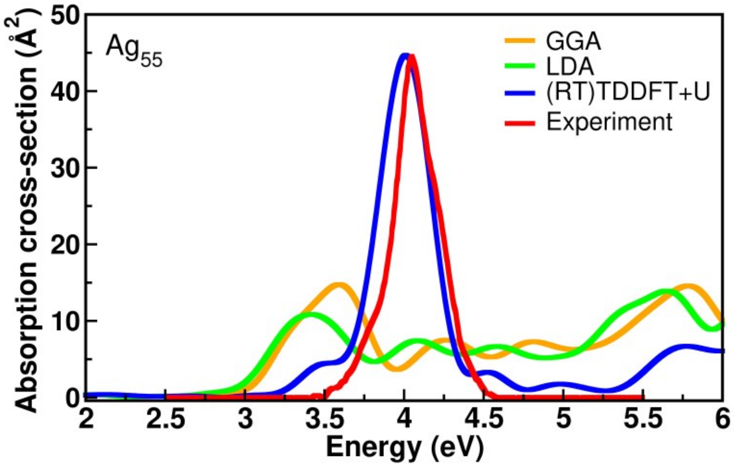


**S3:** Absorption spectra of the $Ag_{55}$ icosahedral cluster using LDA, GGA and TDDFT+U with effective U value of 4 eV, with a total evolution time of ≈ 13 fs (20 $\hbar$/eV). The calculated plasmon energy is strongly underestimated by both the LDA and GGA functionals with many spurious peaks above ≈ 3.5 eV resulting from the overestimation of the intensity and the underestimation of the energy of the interband d→sp transitions. With the effective U correction, the d-electron interband transitions shift to higher energies, resulting in the plasmon band shifting to the correct position, weaker coupling of the LSPR with the interband transitions and, hence, improved agreement with the experiment[3] (red curve) which is blue shifted by 0.17 eV to account for the neon matrix dielectric effect.

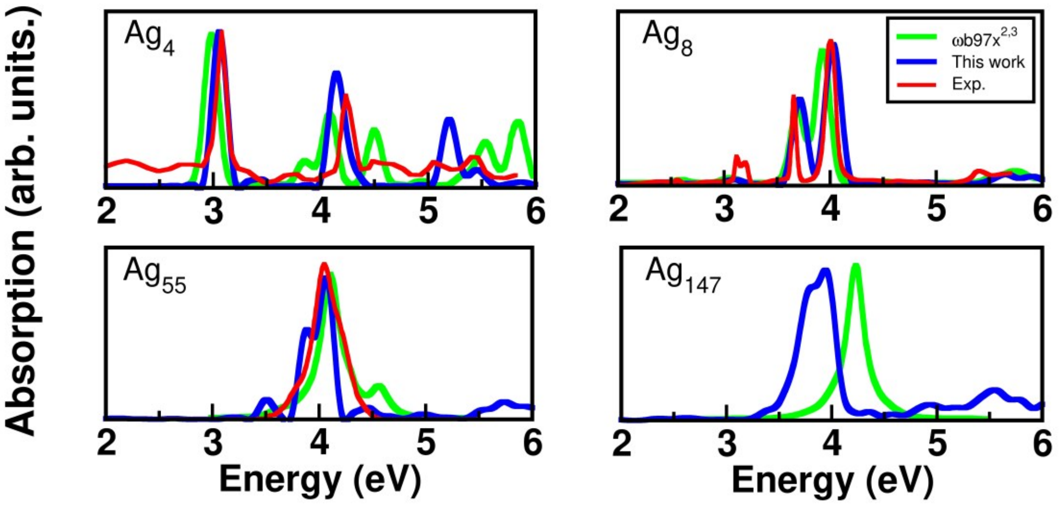


**S4:** Comparison of absorption spectra: red curve ─ experimental data,[4-5] blue curve ─ calculated using TDDFT+U with a total evolution time of ≈ 26 fs (40 ℏ/eV), green curve ─ calculated using DFT with range-separated hybrid functional (RSH) taken from Ref [2,3]. In the case of the $Ag_{147}$ cluster, the difference between the two curves is clearly visible, with the RSH overestimating the plasmon energy by a significant amount. As can be seen in Fig. 3 of the main manuscript, the plasmon energy lies decisively higher than all available experimental results.

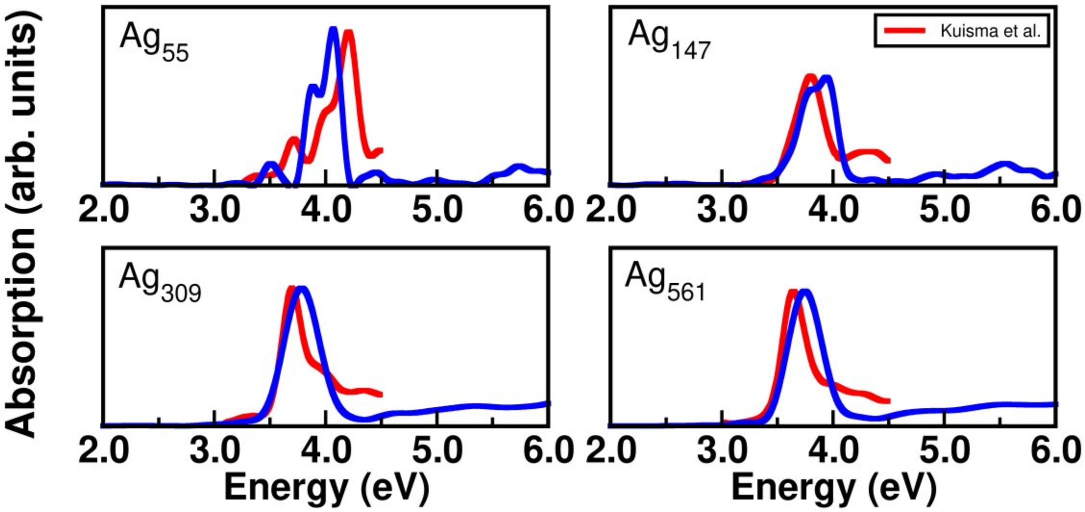


**S5:** Comparison of absorption spectra: blue curve ─ calculated using TDDFT+U, red curve ─ calculated using GLLB-SC, taken from Ref [1]. The calculated spectra shown above are obtained using an evolution time of 26 fs for $Ag_{55}$ and $Ag_{147}$, whereas for $Ag_{309}$ and $Ag_{561}$, an evolution time of 13 fs is used.

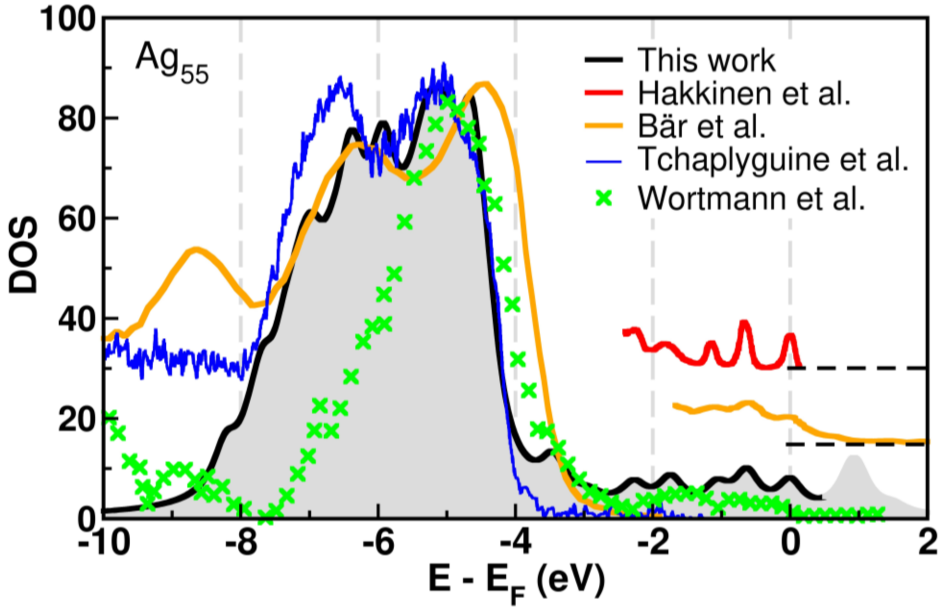


**S6:** Comparison between experimental measured UV photoemission spectra[6-9] and the calculated density of states (DOS) using the DFT+U method for the $Ag_{55}$ icosahedral structure. We remind the reader that these comparisons remain approximate because the results of the modified DFT calculations are not, strictly speaking, excitation energies and can only be considered as such in an approximate manner. The HOMO of the experimental and the calculated curves are adjusted to zero, except in the case of Tchaplyguine *et al.*,[9] for which the HOMO cannot be discerned and the experimental curve (blue) has been shifted to match the edge of the calculated d band. Hakkinen *et al.*[7] and Bär *et al.*[8] experimental curves below the HOMO (red and orange) are stacked vertically for the clear representation. The d band and the states above the d band have been scaled differently in the case of Bär *et al.*[8] The d-band edge in the calculated DOS appears nearly at the correct energy below the HOMO, but the correct width of the band still remains ambiguous. Wortman *et al.* reports a very narrow d band for $Ag_{55}$, measured by depositing the clusters on a graphite substrate, while Bär *et al.*[8] and Tchaplyguine *et al.* directly measure the photoemission spectra in the gas phase and report a broader d band. Somewhat surprisingly, the width of our calculated d band agrees well with the measurement of the non-size selected silver clusters in the gas phase of Tchaplyguine *et al*.[9] In addition, our calculation captures very well all the important features of the occupied states above the d band observed in the UV photoemission spectra[7,8], even though the KS energies are not strictly speaking excitation energies.

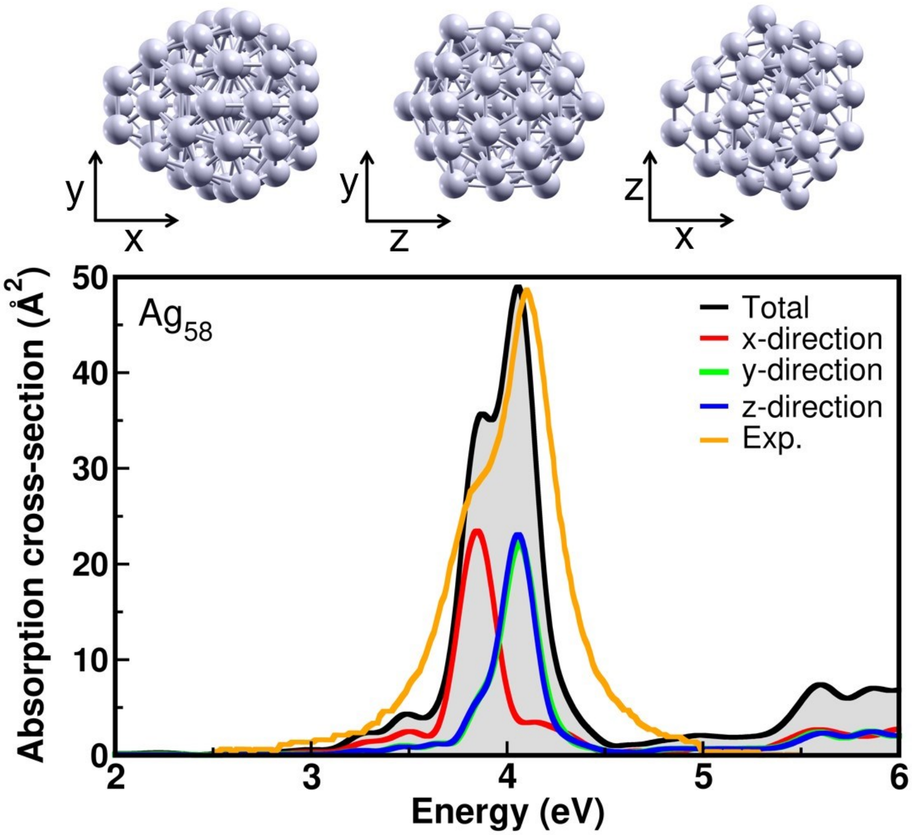


**S7:** Total and direction-resolved calculated absorption cross-section of the $Ag_{58}$ cluster using the TDDFT+U method. Direction-resolved absorption curves confirm that the major contribution to the most intense peak in the total absorption arises from the y and the z-component of the absorption cross-section, while the well-separated shoulder observed at an energy slightly below 4 eV has a major contribution coming from the x-component. Distinguishable and well-separated LSPR energies along the directions result from the deviation of the particle from spherical shape, to one where the aspect ratio plays an important role in determining the position of the LSPR. In the above case, as can be qualitatively seen from the structure presented along three different planes, the particle along the x-direction is longer than along the z or y directions. Since the LSPR modes along the longer axis are lower in energy, the x-direction of the absorption cross-section has its maximum at a lower energy than the other two directions. Hence, for a fixed number of atoms in a cluster (or a fixed volume), the deviation from spherical shape results not only in the broadening but also in shape-dependent shifts and the emergence of extra peaks or shoulders of the LSPR in the total absorption, arising from the splitting of LSPR response along different directions.

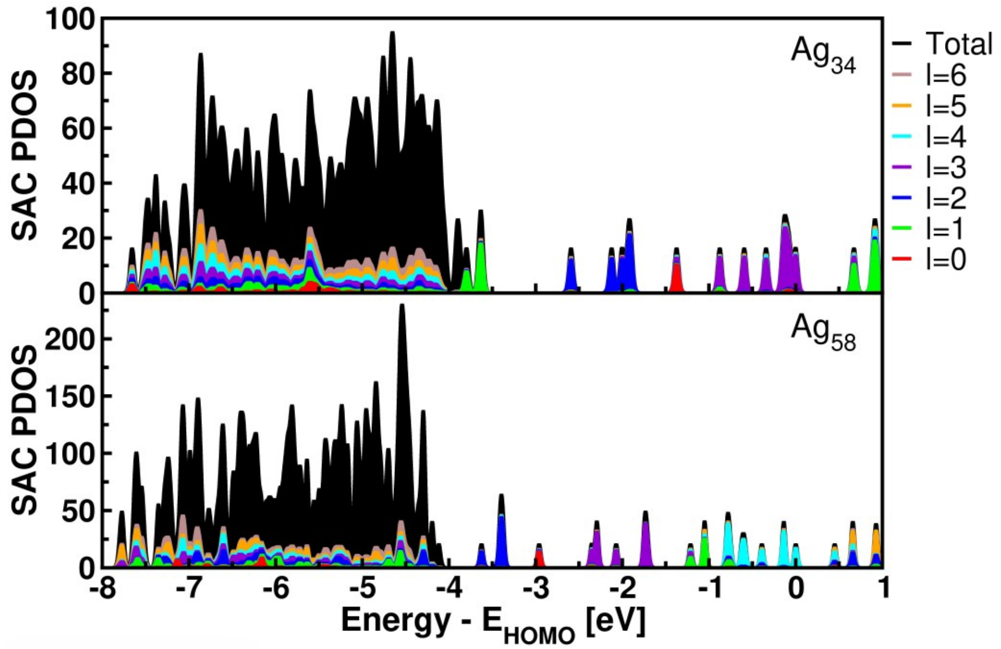


**S8:** The super atom projected density of states for $Ag_{34}$ and $Ag_{58}$ clusters confirms the presence of filled 1F (L=3) and 1G (L=4) shells below the Fermi energy, respectively.

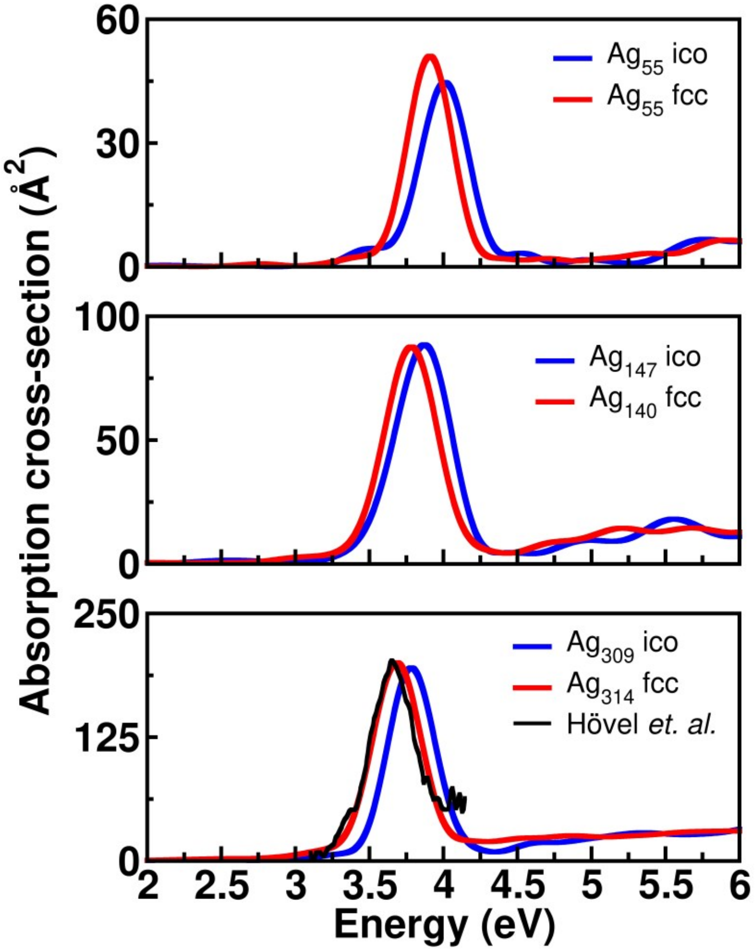


**S9:** Comparison of the absorption spectra of icosahedral and fcc-based Ag clusters of similar sizes, calculated with an evolution time of ≈13 fs (20 $\hbar$/eV). In all the three examples shown above, the absorption spectrum maxima in the fcc-based structures are lower in energy than those of the icosahedral ones. Except for $Ag_{55}$, for which the icosahedral structure is indeed experimentally found and probably the lowest-energy structure,[23] theoretical calculation predicts icosahedral structures to be less favorable compared to fcc-based structures as cluster size increases. This explains that icosahedral clusters, even though very convenient to use, are not necessarily representative for bigger clusters in experiments.

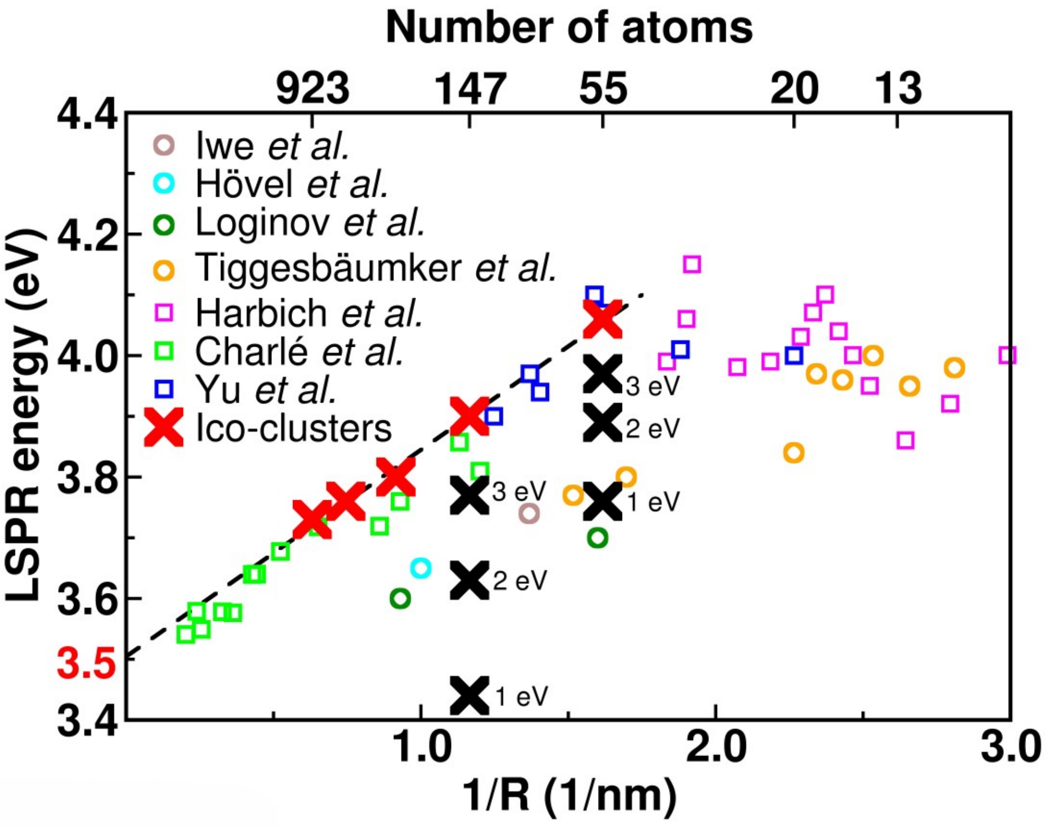


**S10:** Energetic position of LSPR plotted against inverse radius. The calculated points in the above plots are obtained with a simulation radius of 5.0 Å, and a grid spacing of 0.20 Å, respectively. The red crosses are the calculated LSPR position for the icosahedral structures with a effective U value of 4 eV. For $Ag_{55}$ and $Ag_{147}$, further calculations were carried out using smaller effective U values as marked in the above figure. For $Ag_{55}$ and $Ag_{147}$, an effective U value of ≈ 1 and ≈ 2.5 eV results in plasmon energies close to those measured in the free beam experiments.

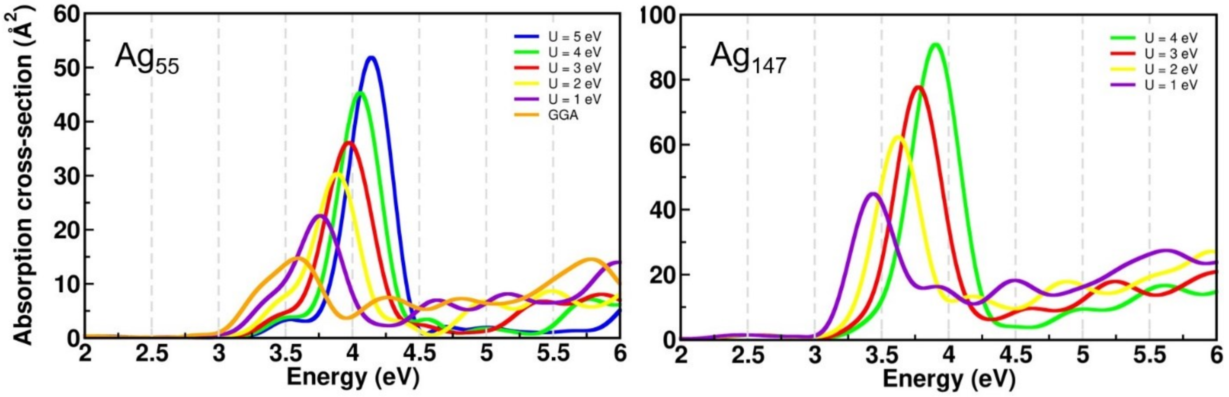


**S11:** Absorption spectra of $Ag_{55}$ and $Ag_{147}$ icosahedral structures, calculated using different effective U values. Spectra are obtained using TDDFT with evolution time of ≈13 fs (20 $\hbar$/eV), with a simulation radius of 5.0 Å

.

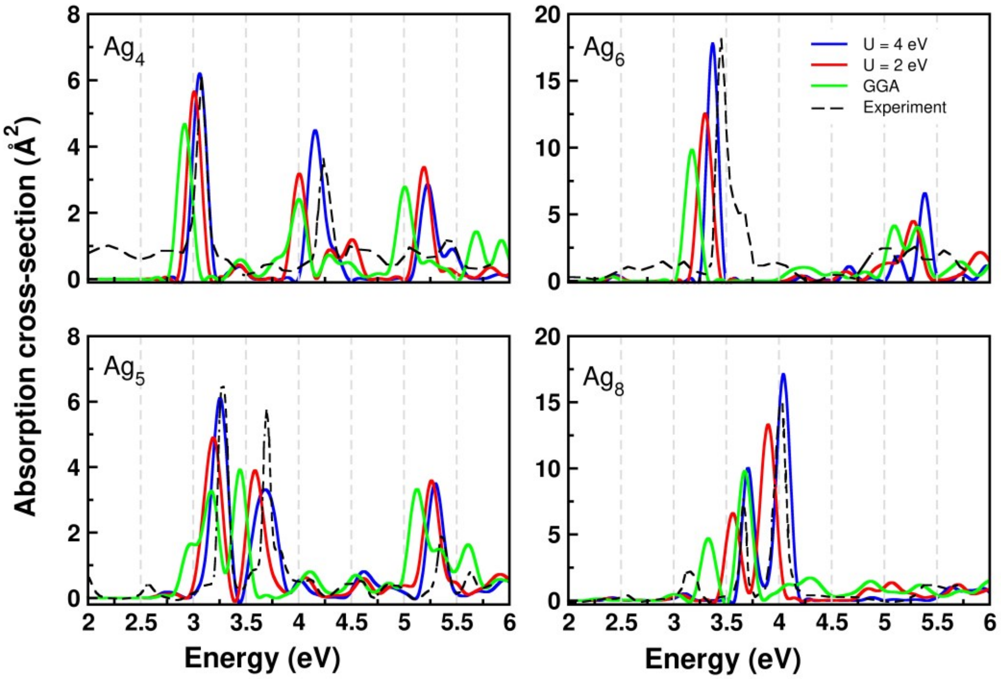


**S12:** Absorption spectra of the small clusters, calculated using different effective U values and compared to unshifted neon-gas matrix experimental results. Notably, when the effective U value is less than 4 eV, the agreement with the experimental data degrades.

## References:


1. Kuisma, M., Sakko, A., Rossi, T. P., Larsen, A. H., Enkovaara, J., Lehtovaara, L., & Rantala, T. T. (2015). Localized surface plasmon resonance in silver nanoparticles: Atomistic first-principles time-dependent density-functional theory calculations. Physical Review B, 91(11), 115431.
2. Rabilloud, F. (2013). Assessment of the performance of long-range-corrected density functionals for calculating the absorption spectra of silver clusters. The Journal of Physical Chemistry A, 117(20), 4267-4278.
3. Schira, R., & Rabilloud, F. (2019). Localized surface plasmon resonance in free silver nanoclusters Ag n, n= 20–147. The Journal of Physsical Chemistry C, 123(10), 6205-6212.
4. Lecoultre, S., Rydlo, A., Buttet, J., Félix, C., Gilb, S., & Harbich, W. (2011). Ultraviolet-visible absorption of small silver clusters in neon: $Ag_n$ (n= 1–9). The Journal of chemical physics, 134(18).
5. Yu, C., Schira, R., Brune, H., von Issendorff, B., Rabilloud, F., & Harbich, W. (2018). Optical properties of size selected neutral Ag clusters: electronic shell structures and the surface plasmon resonance. Nanoscale, 10(44), 20821-20827.
6. Wortmann, B., Mende, K., Duffe, S., Grönhagen, N., von Issendorff, B., & Hövel, H. (2010). Ultraviolet photoelectron spectroscopy of supported mass selected silver clusters. physica status solidi (b), 247(5), 1116-1121.
7. Häkkinen, H., Moseler, M., Kostko, O., Morgner, N., Hoffmann, M. A., & Issendorff, B. V. (2004). Symmetry and electronic structure of noble-metal nanoparticles and the role of relativity. Physical review letters, 93(9), 093401.
8. Bär, F. (2023). High-resolution photoelectron spectroscopy on cold metal clusters (Doctoral dissertation, Dissertation, Universität Freiburg, 2023).
9. Tchaplyguine, M., Peredkov, S., Rosso, A., Schulz, J., Öhrwall, G., Lundwall, M., ... & Björneholm, O. (2007). Direct observation of the non-supported metal nanoparticle electron density of states by X-ray photoelectron spectroscopy. The European Physical Journal D, 45, 295-299.
10. López-Lozano, X., Barron, H., Mottet, C., & Weissker, H. C. (2014). Aspect-ratio-and size-dependent emergence of the surface-plasmon resonance in gold nanorods–an ab initio TDDFT study. Physical Chemistry Chemical Physics, 16(5), 1820-1823.
11. Chen, M., Dyer, J. E., Li, K., & Dixon, D. A. (2013). Prediction of structures and atomization energies of small silver clusters, $Ag_n$, n< 100. The Journal of Physical Chemistry A, 117(34), 8298-8313.
12. Iwe, N., Raspe, K., Martinez, F., Schweikhard, L., Meiwes-Broer, K. H., & Tiggesbäumker, J. (2023). Metal cluster plasmons analyzed by energy-resolved photoemission. Physical Chemistry Chemical Physics, 25(3), 1677-1684.
13. Tiggesbäumker, J., Köller, L., Meiwes-Broer, K. H., & Liebsch, A. (1993). Blue shift of the Mie plasma frequency in Ag clusters and particles. Physical Review A, 48(3), R1749.
14. Haberland, H. (2013). Looking from both sides. Nature, 494(7435), E1-E2.
15. Tiggesbäumker, J., Köller, L., Lutz, H. O., & Meiwes-Broer, K. H. (1992). Giant resonances in silver-cluster photofragmentation. Chemical physics letters, 190(1-2), 42-47.
16. Yamada, A. (2022). Computational Analyses of Plasmonics of a Silver Nanoparticle in a Vacuum and in a Water Solution by Classical Electronic and Molecular Dynamics Simulations. The Journal of Physical Chemistry A, 126(29), 4762-4771.
17. Yeshchenko, O. A., & Pinchuk, A. O. (2021). Thermo-optical effects in plasmonic metal nanostructures. Ukrainian journal of physics, 66(2), 112-112.
18. Baishya, K., Idrobo, J. C., Öğüt, S., Yang, M., Jackson, K., & Jellinek, J. (2008). Optical absorption spectra of intermediate-size silver clusters from first principles. Physical Review B, 78(7), 075439.

19. Loginov, E., Gomez, L. F., Chiang, N., Halder, A., Guggemos, N., Kresin, V. V., & Vilesov, A. F. (2011). Photoabsorption of Ag N (N∼ 6–6000) nanoclusters formed in helium droplets: Transition from compact to multicenter aggregation. Physical review letters, 106(23), 233401.
20. Fedrigo, S., Harbich, W., & Buttet, J. (1992). Media Effects on the Optical Absorption Spectra of Silver Clusters Embedded in Rare Gas Matrices. International Journal of Modern Physics B, 6(23n24), 3767-3771.
21. Gervais, B., Giglio, E., Jacquet, E., Ipatov, A., Reinhard, P. G., & Suraud, E. (2004). Simple DFT model of clusters embedded in rare gas matrix: Trapping sites and spectroscopic properties of Na embedded in Ar. The Journal of chemical physics, 121(17), 8466-8480.
22. Grigoryan, V. G., Springborg, M., Minassian, H., & Melikyan, A. (2013). Optical properties of silver and copper clusters with up to 150 atoms. Computational and Theoretical Chemistry, 1021, 197-205.
23. Schooss, D., Blom, M. N., Parks, J. H., Issendorff, B. V., Haberland, H., & Kappes, M. M. (2005). The structures of ag55+ and ag55-: trapped ion electron diffraction and density functional theory. Nano letters, 5(10), 1972-1977.
24. Hövel, H., Fritz, S., Hilger, A., Kreibig, U., & Vollmer, M. (1993). Width of cluster plasmon resonances: Bulk dielectric functions and chemical interface damping. Physical Review B, 48(24), 18178.
